# Supplementary material for: Selectively Providing Reliance Calibration Cues With Reliance Prediction
Source: arXiv:2302.09995 source file (2023-12-01)
Supplement: Supplementary file 1 [file 99_appendix.tex]

%%
%% If your work has an appendix, this is the place to put it.
\appendix
\section{Links}
A link to the implementation of Trust-former, the reliance dataset, and the experimental results on GitHub will appear after the review phase.
For the review, we included them as supporting files.

\section{CAPTCHA datasets}\label{section:link}
Table~\ref{table:captcha-url} lists the urls for the CAPTCHA datasets used for the CC task.
\begin{table}[h!]
\caption{URLs for the CAPTCHA datasets}\label{table:captcha-url}
\begin{tabular}{l}
URL                                                          \\ \hline
https://www.kaggle.com/datasets/utkarshdoshi/captcha-dataset \\
https://www.kaggle.com/datasets/alizahidraja/captcha-data    \\
https://www.kaggle.com/datasets/kaushikmetha/captcha-images  \\
https://www.kaggle.com/datasets/greysky/captcha-dataset     
\end{tabular}
\end{table}

\section{Environment and hyperparameters}
The task AI and Trust-former were trained on a standard PC with an RTX 3070 GPU and Ryzen 9 5980X CPU.
Table~\ref{table:env} lists the softwares used for training Trust-former.
Table~\ref{table:hyperparameters} shows the hyperparameters of Trust-former.
\begin{table}[h!]
\caption{Softwares}\label{table:env}
\begin{tabular}{c|c}
software & version \\ \hline
python   & 3.8.10  \\
torch    & 1.13.0  \\
numpy    & 1.23.2
\end{tabular}
\end{table}

\begin{table}[h!]
\caption{Hyperparameters}\label{table:hyperparameters}
\begin{tabular}{c|c}
hyperparameter                                             & value \\ \hline
number of Transformer-encoder layers                       & 3     \\
number of Transformer-encoder heasds                       & 16    \\
dimension of Transformer-encoder input                     & 128   \\
dimension of Transformer-encoder \\ feedforward network model & 2048  \\
dropout rate                                               & 0.1   \\
hidden sizes for multi-layer perceptron   & [128, 128, 128]
\end{tabular}
\end{table}
